# Supplementary material for: AutoAD III: The Prequel -- Back to the Pixels
Source: arXiv:2404.14412 source file (2024-04-22)
Supplement: Supplementary file 1 [file supp_metrics.tex]

\begin{table}[h]
\begin{tabular}{|l|l|l|l|l|}
\hline
                                    & AudioVault annotation                                                                                  & Movie-Llama2 Prediction                                  & CRITIC$\uparrow$(0-1) & LLM-AD-Eval$\uparrow$(0-5) \\ \hline
\multirow{4}{*}{Sherlock Holmes}    & Holmes follows her around a corner.                                                                    & Holmes follows her.                                      & 1.0    & 5           \\ \cline{2-5} 
                                    & Mary is in her late thirties with a mop of curly red hair under her black veil.                        & The carriage pulls up outside a narrow alleyway.         & 0.0    & 0           \\ \cline{2-5} 
                                    & Dazed, he lifts up his head.                                                                           & He lies on the ground, his head twisted at an odd angle. & 1.0    & 4           \\ \cline{2-5} 
                                    & His vision is blurred, but he sees a man scoop Mary up off the road and drag her towards the carriage. & He falls to the ground.                                  & 1.0    & 4           \\ \hline
\multirow{3}{*}{Back to the Future} & Marty's speedometer tops at a stop sign, he turns hard right.                                          & Marty's car speeds down the road.                        & 1.0    & 2           \\ \cline{2-5} 
                                    & Marty's radiation helmet falls over his head as the car zooms in the barn door.                        & The car speeds through the barn and out the other side.  & 0.0    & 2           \\ \cline{2-5} 
                                    & George rides through the square on a bicycle, and Marty bursts out of the cafe after him.              & Marty rides his bike out of the diner.                   & 1.0    & 4           \\ \hline
\end{tabular}
\end{table}
